# Supplementary material for: Iris Recognition After Death
Source: arXiv:1804.01962 ancillary file (2018-10-31)
Supplement: Supplementary file 1 [file IrisRecognitionAfterDeath-TIFS-supplementaryMaterial.pdf]

# Supplementary material

## Iris Recognition After Death

Mateusz Trokielewicz, Adam Czajka, Piotr Maciejewicz

October 31, 2018

This supplementary material contains an analysis of selected ISO image quality metrics [1] calculated for images from the Warsaw-BioBase-Post-Mortem-Iris-v2, together with statistical analysis in respect to time elapsed since death, and example images for several different irises and post-mortem time horizons.

## 1 ISO/IEC iris image quality metrics

The ISO/IEC 29794-6 standard on iris image quality [1] defines a series of quality metrics suggested to which iris images used in a biometric system should comply. Two of those metrics can be calculated using a raw iris image, without the additional information regarding iris location in the image, namely: *Grayscale utilisation* (image histogram entropy), and *Sharpness*. These covariates are defined as follows:

- *Grayscale utilization*, or the entropy of the iris image histogram  $H$  measured in bits, examines pixel values of an iris image to calculate a spread of intensity values and assess whether the image is properly exposed:

$$H = - \sum_{i=1}^{256} p_i \log_2 p_i$$

where  $p_i$  is the probability of each gray level  $i$  occurring in the image, hence, the total count of pixels at gray level  $i$ , divided by the total number of pixels in the image [1];

- *Sharpness*, determined by the power resulting from filtering the image with a Laplacian of Gaussian kernel; for brevity, we do not reproduce the formulae here, and instead refer the Reader to the original ISO/IEC documentation [1].

## 2 Statistical representations

In Figs. 1 through 4 we include boxplots representing the two metrics defined above in respect to the type of image, namely near-infrared (NIR) and red channel of the RGB images (R). In either case, no clear trends are observable for any of the covariates.

## 3 Example images and corresponding scores

Figs. 5 through 8 present selected NIR and R samples collected from two different subjects at different moments after death, together with their corresponding quality scores.

## References

- [1] ISO/IEC 29794-6, “Information technology – Biometric sample quality - Part 6: Iris image data (FDIS),” August 2014.

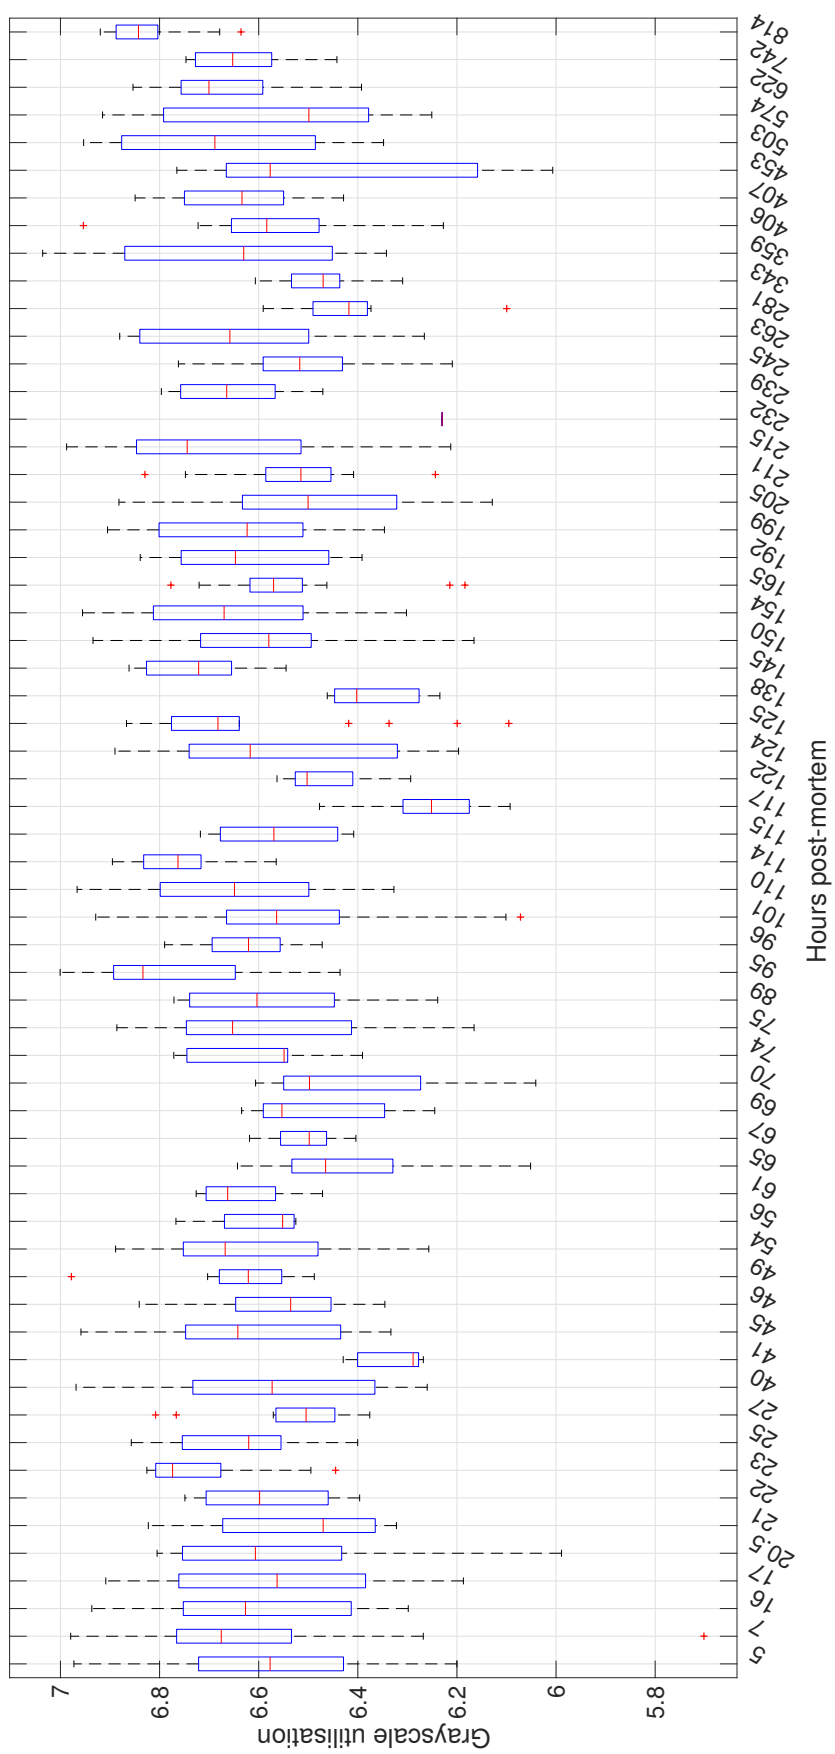

Figure 1: *Grayscale utilisation* calculated for NIR images, plotted in the form of boxplots against time interval post-mortem.

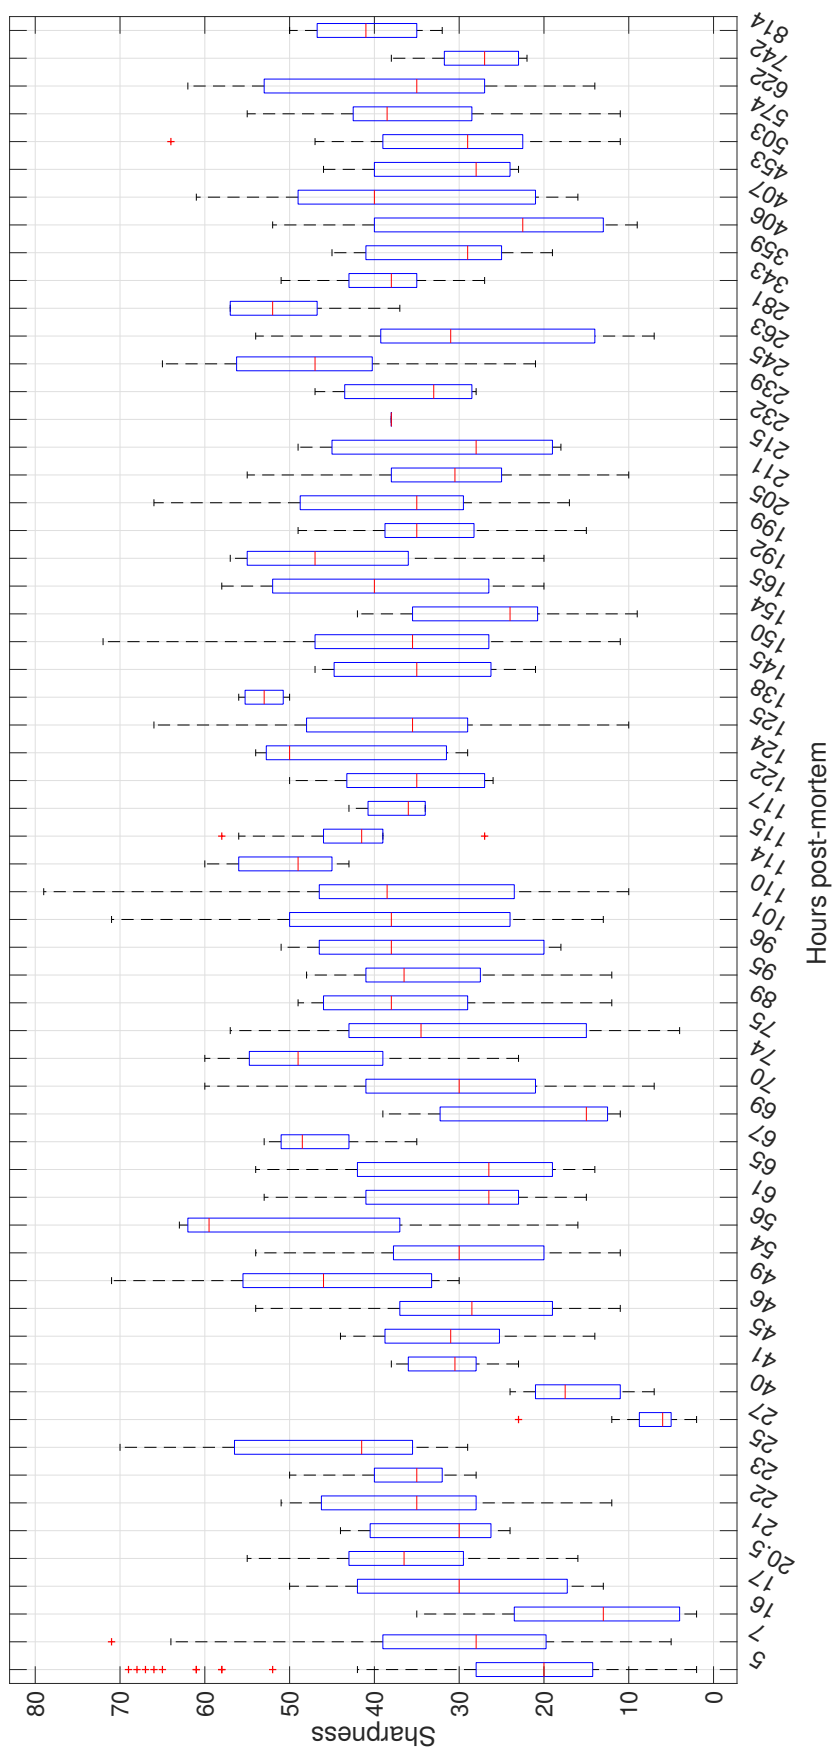

Figure 2: *Sharpness* calculated for NIR images, plotted in the form of boxplots against time interval post-mortem.

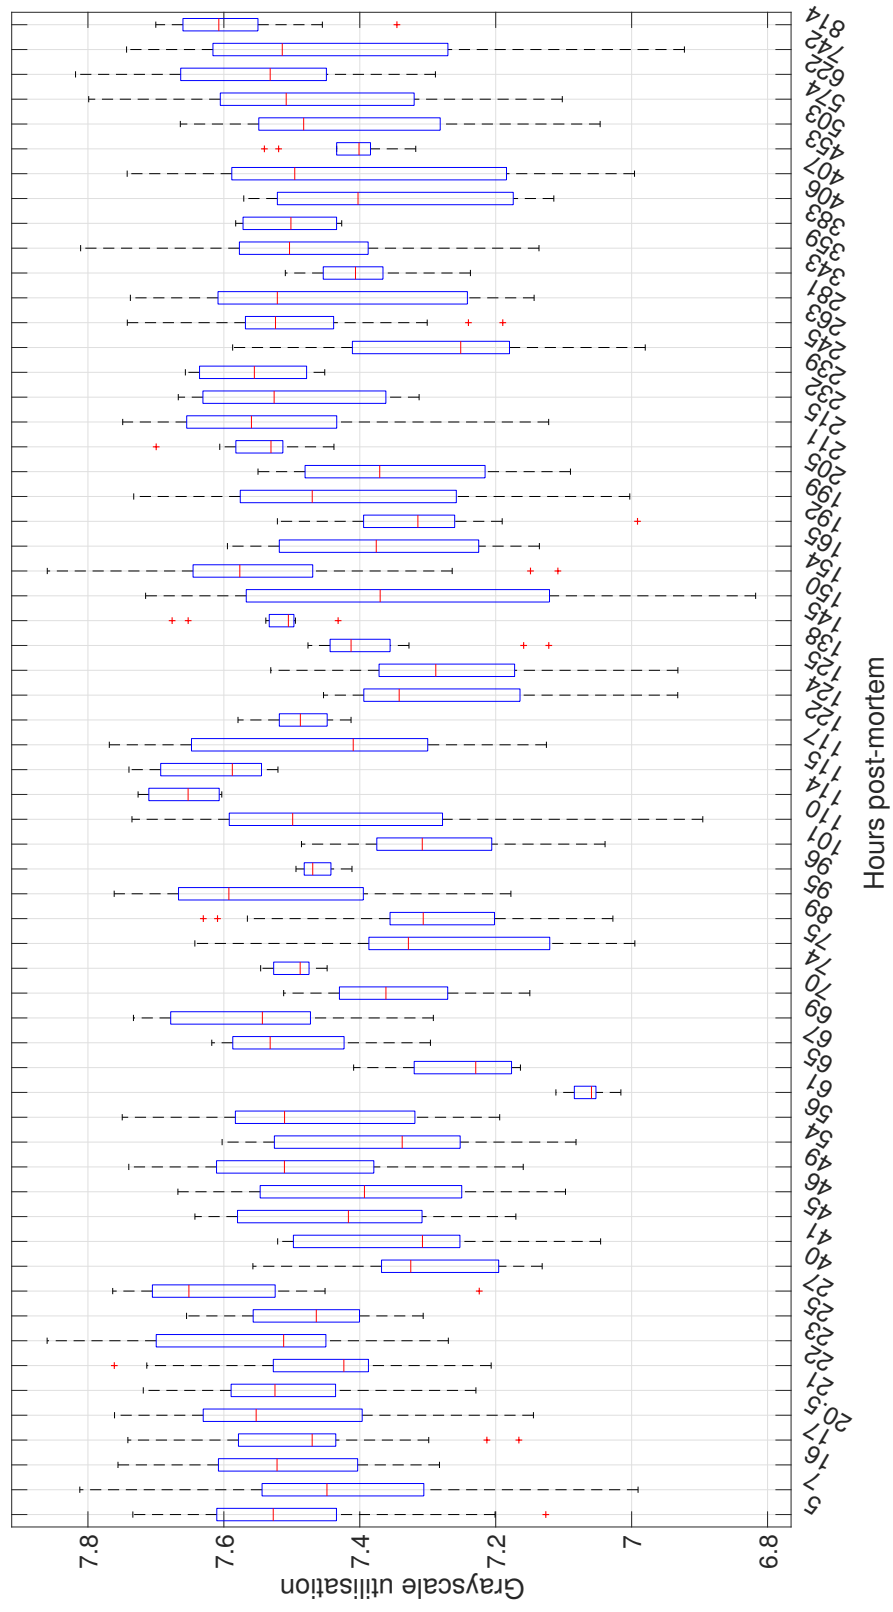

Figure 3: *Grayscale utilisation* calculated for R images, plotted in the form of boxplots against time interval post-mortem.

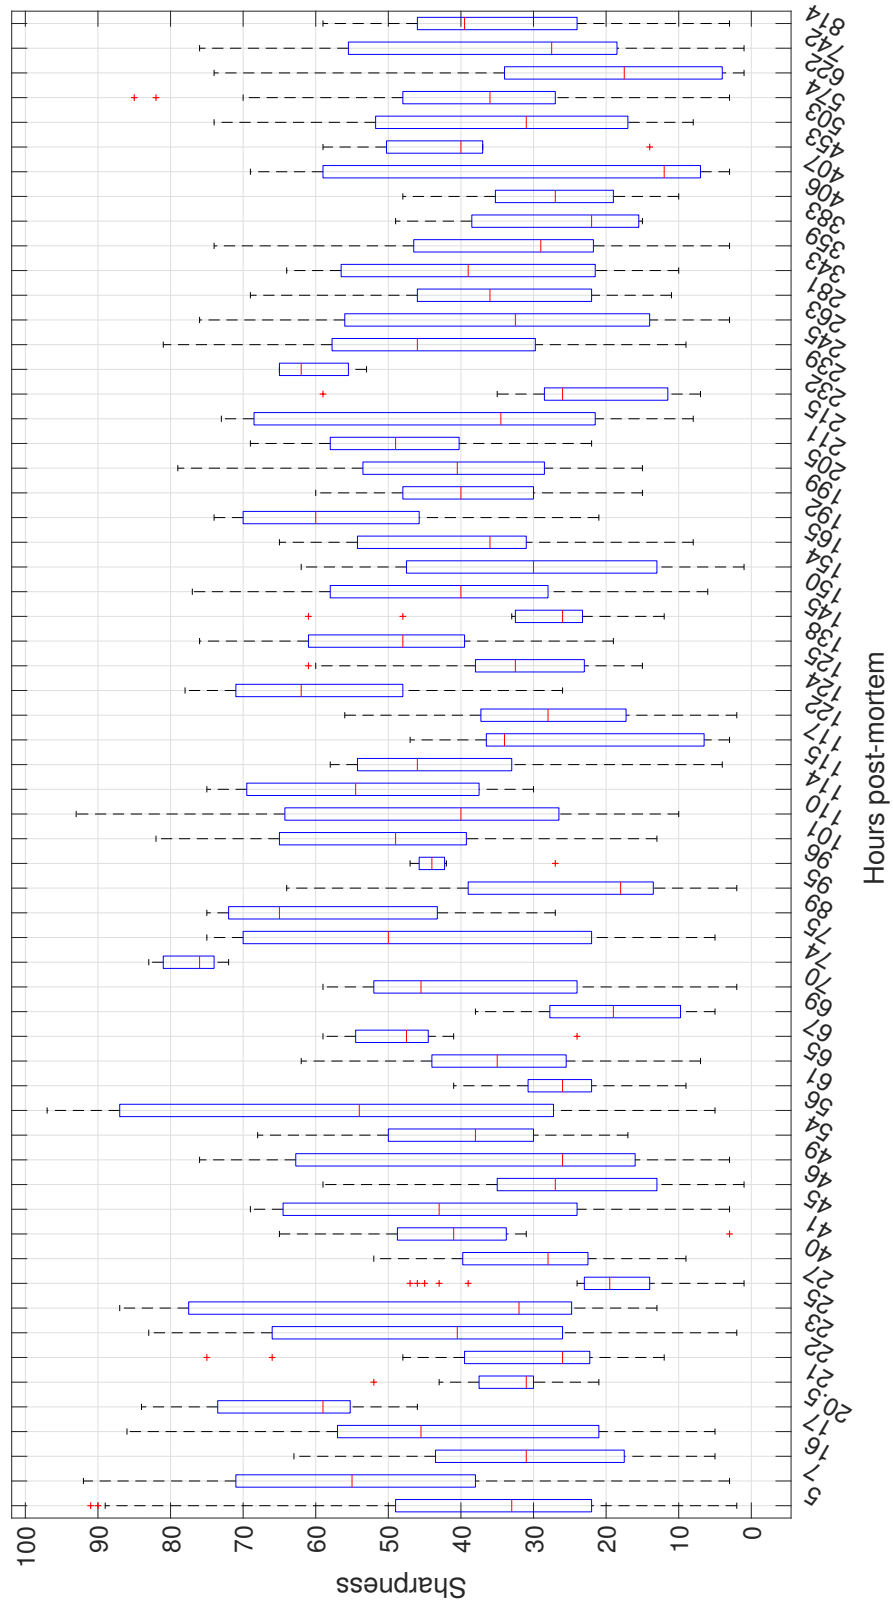

Figure 4: Sharpness calculated for R images, plotted in the form of boxplots against time interval post-mortem.

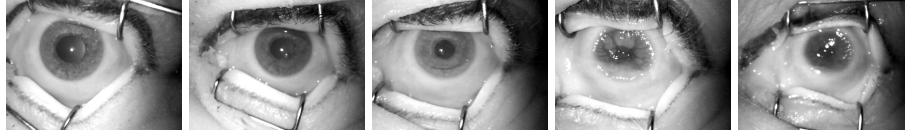

(a) time: 5h      (b) time: 23h      (c) time: 263h      (d) time: 574h      (e) time: 814h  
 GU: 6.90      GU: 6.82      GU: 6.88      GU: 6.79      GU: 6.83  
 SH: 25      SH: 36      SH: 27      SH: 43      SH: 39

**Figure 5:** NIR images of subject 0017, left eye. *Grayscale utilisation* (GU) and *sharpness* (SH) covariates are given, together with time elapsed since death.

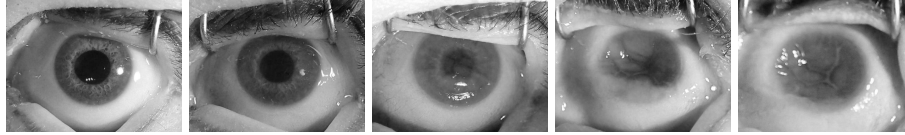

(a) time: 5h      (b) time: 23h      (c) time: 263h      (d) time: 574h      (e) time: 814h  
 GU: 7.70      GU: 7.45      GU: 7.52      GU: 7.50      GU: 7.55  
 SH: 49      SH: 60      SH: 61      SH: 56      SH: 8

**Figure 6:** Same as in Fig. 5, but for R images.

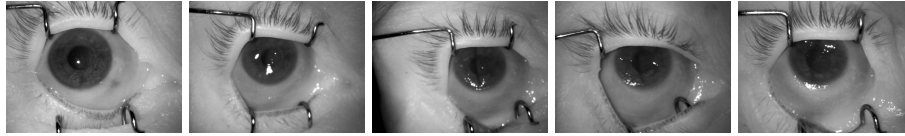

(a) time: 7h      (b) time: 89h      (c) time: 192h      (d) time: 232h      (e) time: 281h  
 GU: 6.27      GU: 6.24      GU: 6.64      GU: 6.23      GU: 6.10  
 SH: 48      SH: 49      SH: 47      SH: 38      SH: 57

**Figure 7:** Same as in Fig. 5, but for samples collected from the right eye of subject 0102.

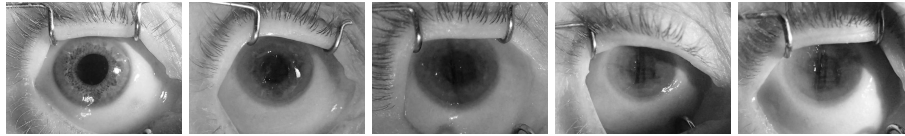

(a) time: 7h      (b) time: 89h      (c) time: 192h      (d) time: 232h      (e) time: 281h  
 GU: 7.54      GU: 7.25      GU: 7.19      GU: 7.60      GU: 7.72  
 SH: 69      SH: 43      SH: 21      SH: 26      SH: 19

**Figure 8:** Same as in Fig. 7, but for R images.
